# Supplementary material for: Training invariances and the low-rank phenomenon: beyond linear networks
Source: arXiv:2201.11968 source file (2022-04-26)
Supplement: Supplementary file 1 [file appendixD.tex]

\section{Extension to gradient descent}
Recall that with gradient descent for some step size $\eta: \mathbb{N} \to \R_{\geq 0}$, the weight trajectory is a solution to the system of finite differences: 
\begin{equation}\label{eqn:gd}
  w(t + 1) - w(t) = -\eta(t) d(w(t)),
\end{equation}
for some $\{d(w(t)) \in \partial\cR(w(t))\}_{t \in \mathbb{N}}$ sequence of subgradient choice at each time step. This section essentially recovers \citet{jitel_alignment} extension of deep linear network results to gradient descent. 

From \ref{eqn:gd}, for some $\{d(w(t)) \in \partial\cR(w(t))\}_{t \in \mathbb{N}}$, we have,
\begin{align}
  w(t + 1)w(t) - w(t)^2 &= -\eta(t) w(t) d(w(t))\\
  w(t+1)^2 + w(t)^2 - 2 w(t + 1)w(t) &= \eta(t)^2 d(w(t))^2, 
\end{align} by multiplying both sides with $w(t)$ or squaring both sides respectively.

Combine the above two equations to get: 
 \begin{equation}
   w(t + 1)^2 - w(t)^2 - \eta(t)^2 d(w(t))^2  = - 2 \eta(t) w(t) d(w(t)).
\end{equation}

Take a telescoping sum to get:
\begin{equation}
  w(t+1)^2 - w(0)^2 - \sum_{\tau = 0}^t \eta(\tau)^2 d(w(\tau))^2 = -2\sum_{\tau = 0}^t \eta(\tau) w(\tau) d(w(\tau)).
\end{equation}

Fix an edge $e$ and recall that we had from the proof of Theorem \ref{thm:matrix-wise_invariance} that, for all $s \in  \mathbb{N}$,
\begin{align}
  w_e(s) [d(w(s))]_{e} = \sum_{p \in \cP | e \in p} \frac{1}{n} \sum_{j = 1}^n d_{j,p}(w(s)).
\end{align}

Therefore, fix a vertex $v$ satisfying the conditions in Theorem \ref{thm:matrix-wise_invariance}, we have,
 \begin{align}
   &\sum_{u \in \IN_v} w_{uv}(t+1)^2 - w_{uv}(0)^2 - \sum_{\tau = 0}^t \eta(\tau)^2 [d(w(\tau))]_{uv}^2 \\
   =&-2 \sum_{\tau = 0}^t \eta(\tau) \sum_{p \in \cP | v \in p} \frac{1}{n} \sum_{j = 1}^n d_{j,p}(w(\tau))\\
   =& \sum_{b \in \IN_v} w_{vb}(t+1)^2 - w_{vb}(0)^2 - \sum_{\tau = 0}^t \eta(\tau)^2 [d(w(\tau))]_{vb}^2.
 \end{align}  which recovers a vertex-wise invariance with some slack terms. With an identical argument, we can recover the second part of Theorem \ref{thm:matrix-wise_invariance} as well:
 \begin{align}
   &\sum_{a \in \IN} w_{av}(t+1)w_{au}(t+1) - w_{av}(0)w_{au}(0) - \sum_{\tau = 0}^t \eta(\tau)^2 [d(w(\tau))]_{av} [d(w(\tau))]_{au} \\
   =&-2\sum_{\tau = 0}^t \eta(\tau) \sum_{a \in \IN} w_{av}(\tau) [d(w(\tau))]_{au} + w_{au}(\tau) [d(w(\tau))]_{av}\\
   =&-2 \sum_{\tau = 0}^t \eta(\tau) \sum_{p \in \cA} \frac{1}{n} \sum_{j = 1}^n d_{j,p}(w(\tau))\\
   =&-2\sum_{\tau = 0}^t \eta(\tau) \sum_{b \in \OUT} w_{vb}(\tau) [d(w(\tau))]_{ub} + w_{ub}(\tau) [d(w(\tau))]_{bv}\\
   =& \sum_{b \in \IN_v} w_{vb}(t+1)w_{ub}(t+1) - w_{vb}(0)w_{ub}(0) - \sum_{\tau = 0}^t \eta(\tau)^2 [d(w(\tau))]_{vb}[d(w(\tau))]_{ub}.
 \end{align}

  We thus recover the matrix invariance of \citet{jitel_alignment} equation C.9. 

 To control singular values of adjacent layers' matrix representations, we need to control the growth of the slack term using the step size $\eta$. One way to do this is to adaptively set the step size based on the Frobenius norm of each layer. Let us assume that at time step  $t$, the maximum Frobenius norm of any layer is  $R(t)$ and that the risk $\cR$ (as a function of time) has  $\beta(t)$-Lipschitz gradient (or is  $\beta(t)$-smooth) in this Frobenius norm ball. Then by smoothness of  $\cR$, setting $\eta(\tau) = \min\left(1,\dfrac{1}{\beta(\tau)}\right)$ for any $\tau \in \mathbb{N} $, we have,
 \begin{align}
   \cR(w(\tau+1)) - \cR(w(\tau)) &\leq \ip{d(w(\tau))}{-\eta(t) d(w(\tau))} + \frac{\beta(\tau)\eta(\tau)^2}{2} \|d(w(\tau))\|_2^2\\
                               &=-\frac{\eta(\tau)}{2} \|d(w(\tau))\|_2^2.
 \end{align}

 Therefore,
\begin{align}
  -\cR(w(0)) \leq  \cR(w(t + 1)) - \cR(w(0))&\leq -\frac{1}{2} \sum_{\tau = 0}^t \eta(\tau) \|d(w(\tau))\|_2^2\\
                                           &\leq -\frac{1}{2} \sum_{\tau = 0}^t \eta(\tau)^2 \|d(w(\tau))\|_2^2\\
                                           &\leq -\left|\sum_{\tau = 0}^t \eta(\tau)^2 [d(w(\tau))]_e [d(w(\tau))]_f\right|.
\end{align} for any $e,f \in E$. Therefore we conclude that the slack term is bounded by a quantity that is fixed at initialization. This allows us to recover Theorem \ref{thm:low_rank_non_homogeneous} and Corollary \ref{thm:low_rank} for gradient descent (but note that here we have an extra assumption in term of the smoothness of the risk function).
